# Supplementary material for: Modelling size distributions of marine plastics under the influence of continuous cascading fragmentation
Source: arXiv:2011.01775 ancillary file (2020-11-03)
Supplement: Supplementary file 1 [file Supplementary_material.pdf]

# Supplementary Material: Modelling size distributions of marine plastics under the influence of continuous cascading fragmentation

Mikael L. A. Kaandorp, Henk A. Dijkstra, Erik van Sebille

November 3, 2020

## S1 Additional results: parameter settings and Mass Size Distributions (MSDs)

The main text presents the transient NSD results for the baseline scenario, and various steady state NSD results for scenarios where model parameters are varied. An overview of the box model parameters is given in table S1. The corresponding MSDs are presented in figure S1. Results show clearly that the scenarios have a strong effect on the estimated mass for given particle sizes. Increased fragmentation, either resulting from increased fragmentation rates or increased transport towards beaches, results in the smaller particles making up more of the total mass. The results of these simulations should be verified in the future with more in-situ measurements, as this will give us more insight in the marine plastic mass budget.

Table S1: Environmental box model parameters used to simulate the PSDs in figure 6 and figure 7 of the main text, and figure S1. Transition probabilities are given per week.

| | Baseline | Size-dependent ocean transport | Size-dependent re-suspension | Increased frag. | Increased input | fig.7 main text |
|---|---|---|---|---|---|---|
| $\mathbf{P_{O,O}}$ | $7.2 \cdot 10^{-1}$ | $7.3\cdot 10^{-1}$–$8.7\cdot 10^{-1}$ | $7.2 \cdot 10^{-1}$ | $7.2 \cdot 10^{-1}$ | $6.5 \cdot 10^{-1}$ | $7.4\cdot 10^{-1}$–$8.8\cdot 10^{-1}$ |
| $\mathbf{P_{O,C}}$ | $2.7\cdot 10^{-1}$ | $1.2\cdot 10^{-1}$–$2.6\cdot 10^{-1}$ | $2.7\cdot 10^{-1}$ | $2.7\cdot 10^{-1}$ | $2.4\cdot 10^{-1}$ | $1.2\cdot 10^{-1}$–$2.6\cdot 10^{-1}$ |
| $\mathbf{P_{C,O}}$ | $3.4\cdot 10^{-2}$ | $3.2\cdot 10^{-2}$–$3.4\cdot 10^{-2}$ | $3.4\cdot 10^{-2}$ | $3.4\cdot 10^{-2}$ | $3.0\cdot 10^{-2}$ | $3.2\cdot 10^{-2}$–$3.4\cdot 10^{-2}$ |
| $\mathbf{P_{C,C}}$ | $8.3\cdot 10^{-1}$ | $8.3\cdot 10^{-1}$–$8.3\cdot 10^{-1}$ | $8.3\cdot 10^{-1}$ | $8.3\cdot 10^{-1}$ | $7.4\cdot 10^{-1}$ | $8.4\cdot 10^{-1}$–$8.4\cdot 10^{-1}$ |
| $\mathbf{P_{C,B}}$ | $1.3\cdot 10^{-1}$ | $1.3\cdot 10^{-1}$ | $1.3\cdot 10^{-1}$ | $1.3\cdot 10^{-1}$ | $1.2\cdot 10^{-1}$ | $1.3\cdot 10^{-1}$ |
| $\mathbf{P_{B,C}}$ | $3.2\cdot 10^{-2}$ | $3.2\cdot 10^{-2}$ | $2.0\cdot 10^{-3}$–$4.5\cdot 10^{-1}$ | $3.2\cdot 10^{-2}$ | $2.9\cdot 10^{-2}$ | $2.0\cdot 10^{-3}$–$4.5\cdot 10^{-1}$ |
| $\mathbf{P_{B,B}}$ | $9.6\cdot 10^{-1}$ | $9.6\cdot 10^{-1}$ | $5.5\cdot 10^{-1}$–$9.9\cdot 10^{-1}$ | $9.6\cdot 10^{-1}$ | $8.6\cdot 10^{-1}$ | $5.5\cdot 10^{-1}$–$9.9\cdot 10^{-1}$ |
| **$\lambda$ [f week$^{-1}$]** | $1.8\cdot 10^{-2}$ | $1.8\cdot 10^{-2}$ | $1.8\cdot 10^{-2}$ | $3.3\cdot 10^{-1}$ | $1.8\cdot 10^{-2}$ | $1.0\cdot 10^{-2}$ |
| **input [t yr$^{-1}$]** | 2,500 | 2,500 | 2,500 | 2,500 | 100,000 | 2,500 |
| $\mathbf{P_{S}}$ | $5.1\cdot 10^{-3}$ | $5.1\cdot 10^{-3}$ | $5.6\cdot 10^{-4}$ | $5.1\cdot 10^{-3}$ | $1.1\cdot 10^{-1}$ | $5.0\cdot 10^{-4}$ |

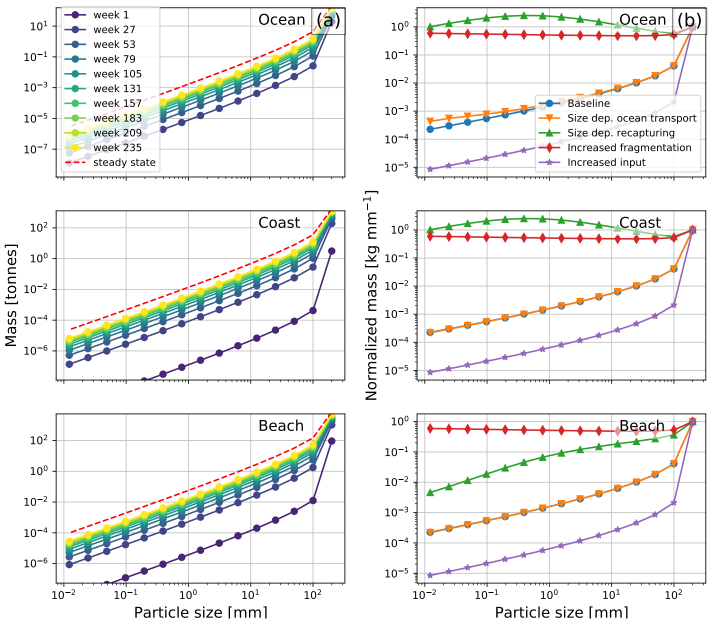


Figure S1: Modelling MSDs using the environmental box model. Column a: transient response to a constant input of particles into the model (baseline scenario). Column b: steady state normalized MSDs for different environmental scenarios, normalized to the amount of parent particles (200 mm)

## S2 Box model: transition matrix formulation

In this section we describe how the transition matrix underlying the environmental box model is set up, and how the steady-state is calculated. As explained in the main text, the transition matrix captures the effect of transport in the environment, as well as the effect of fragmentation. The transition matrix describes these effects for a given time step, set to one week. As a simple example, we present the case where the fragmentation rate $\lambda$ is $1\,f$ week$^{-1}$, and we take $p = 0.5$, $D_N = 3$. For size class $k = 0, 1, 2...$ the cascading fragmentation model at $f = 1$ yields in terms of abundance $n = 0.5, 2, 8...$ fragments per parent particle, and in terms of mass fractions $m = \frac{1}{2}, \frac{1}{4}, \frac{1}{8}....$

The transition matrix in terms of abundance ($\mathbf{T}_n$) is presented in figure S2, the one in terms of mass ($\mathbf{T}_m$) in figure S3. The example is shown for three different size classes only. For notation, we use O, C, and B to denote ocean, coast, and beach respectively, subscripts are used to denote the size class $k$, superscripts are used for time indices $i$. On the left hand side of figure S2 and figure S3, we have the abundance or mass at time $i+1$, on the right hand side we have the transition matrix multiplying the abundance or mass at time $i$. Cells in the transition matrix containing zeros are left empty. The two coloured blocks (red and yellow) indicate the entries where fragmentation is active. As can be seen the matrix is quite sparse. This is because fragmentation is only active on the beach, so particles do not move from one size class to another in the coastal water or ocean. On the beach, particles can move to a higher or equal size class $k$ under influence of fragmentation. The upper right entries of the red and yellow blocks are zero, since particles can not move to a lower size class (i.e. they cannot increase in size). If one has an infinite amount of size classes, the operation in figure S3 would be mass conserving. Due to a finite amount of size classes, there is some mass loss due to fragmentation however. Finally, the entire transition matrices in figure S2 and figure S3 are multiplied with the scalar $P_S$, as particles are removed from the system by sinks (e.g. plastic particles sinking down, or being removed from beaches). As explained in the main, text $P_S$ is assumed to be the same in all environmental boxes, however this value could be varied per environmental box if indications for this become available in future studies.

Size-dependent transport is easily added to the transition matrix, by varying the transition probabilities per size class. All columns are properly normalized (i.e. column sums of 1), such that there would be conservation of mass when there would be no fragmentation or sinks in the system.

Since there is a constant input of new parent objects into the system, the mass at time $i+1$ is given by the mass at time $i$ and the addition of new mass $\mathbf{m}_{in}$:

$$\mathbf{m}^{i+1} = \mathbf{T}_m \mathbf{m}^i + \mathbf{T}_m \mathbf{m}_{in} \tag{1}$$

We want to estimate the steady state mass of the box model ($\mathbf{m}^{ss}$), which is done by setting

$$\mathbf{m}^{i+1} = \mathbf{m}^i = \mathbf{m}^{ss}, \tag{2}$$

$$
\begin{bmatrix} O, n_{k=0}^{i+1} \\ O, n_{k=1}^{i+1} \\ O, n_{k=2}^{i+1} \\ C, n_{k=0}^{i+1} \\ C, n_{k=1}^{i+1} \\ C, n_{k=2}^{i+1} \\ B, n_{k=0}^{i+1} \\ B, n_{k=1}^{i+1} \\ B, n_{k=2}^{i+1} \end{bmatrix}
=
\begin{bmatrix}
P_{O,O} & & & P_{C,O} & & & & & \\
 & P_{O,O} & & & P_{C,O} & & & & \\
 & & P_{O,O} & & & P_{C,O} & & & \\
P_{O,C} & & & P_{C,C} & & & 1/2 * P_{B,C} & & \\
 & P_{O,C} & & & P_{C,C} & & 2 * P_{B,C} & 1/2 * P_{B,C} & \\
 & & P_{O,C} & & & P_{C,C} & 4 * P_{B,C} & 2 * P_{B,C} & 1/2 * P_{B,C} \\
 & & & P_{C,B} & & & 1/2 * P_{B,B} & & \\
 & & & & P_{C,B} & & 2 * P_{B,B} & 1/2 * P_{B,B} & \\
 & & & & & P_{C,B} & 4 * P_{B,B} & 2 * P_{B,B} & 1/2 * P_{B,B}
\end{bmatrix}
\begin{bmatrix} O, n_{k=0}^{i} \\ O, n_{k=1}^{i} \\ O, n_{k=2}^{i} \\ C, n_{k=0}^{i} \\ C, n_{k=1}^{i} \\ C, n_{k=2}^{i} \\ B, n_{k=0}^{i} \\ B, n_{k=1}^{i} \\ B, n_{k=2}^{i} \end{bmatrix}
* P_S
$$

Figure S2: Box model transition matrix in terms of abundance, for three different size classes $k = 0, 1, 2$, and after $f = 1$

$$
\begin{bmatrix} O, m_{k=0}^{i+1} \\ O, m_{k=1}^{i+1} \\ O, m_{k=2}^{i+1} \\ C, m_{k=0}^{i+1} \\ C, m_{k=1}^{i+1} \\ C, m_{k=2}^{i+1} \\ B, m_{k=0}^{i+1} \\ B, m_{k=1}^{i+1} \\ B, m_{k=2}^{i+1} \end{bmatrix}
=
\begin{bmatrix}
P_{O,O} & & & P_{C,O} & & & & & \\
 & P_{O,O} & & & P_{C,O} & & & & \\
 & & P_{O,O} & & & P_{C,O} & & & \\
P_{O,C} & & & P_{C,C} & & & 1/2 * P_{B,C} & & \\
 & P_{O,C} & & & P_{C,C} & & 1/4 * P_{B,C} & 1/2 * P_{B,C} & \\
 & & P_{O,C} & & & P_{C,C} & 1/8 * P_{B,C} & 1/4 * P_{B,C} & 1/2 * P_{B,C} \\
 & & & P_{C,B} & & & 1/2 * P_{B,B} & & \\
 & & & & P_{C,B} & & 1/4 * P_{B,B} & 1/2 * P_{B,B} & \\
 & & & & & P_{C,B} & 1/8 * P_{B,B} & 1/4 * P_{B,B} & 1/2 * P_{B,B}
\end{bmatrix}
\begin{bmatrix} O, m_{k=0}^{i} \\ O, m_{k=1}^{i} \\ O, m_{k=2}^{i} \\ C, m_{k=0}^{i} \\ C, m_{k=1}^{i} \\ C, m_{k=2}^{i} \\ B, m_{k=0}^{i} \\ B, m_{k=1}^{i} \\ B, m_{k=2}^{i} \end{bmatrix}
* P_S
$$

Figure S3: Box model transition matrix in terms of mass, for three different size classes $k = 0, 1, 2$, and after $f = 1$

which yields:

$$\mathbf{m}^{ss} - \mathbf{T}_m \mathbf{m}^{ss} = \mathbf{T}_m \mathbf{m}_{in} \tag{3}$$

$$\mathbf{m}^{ss} = (\mathbf{I} - \mathbf{T}_m)^{-1} \mathbf{T}_m \mathbf{m}_{in}. \tag{4}$$

The transition matrix $\mathbf{T}_m$ has one unknown parameter, $P_S$. This value is optimized such that the steady state floating mass is equal to the midpoint estimate for the Mediterranean sea by Cózar et al. (2015) (2,000 metric tonnes).

# S3 Vertical mixing and size-dependent lateral transport

## S3.1 Modelling mixing and Stokes drift

Vertical mixing of plastic particles is estimated using the approach from Poulain et al. (2019). The rise velocity $w_b$ is estimated by solving (Poulain et al., 2019; Clift et al., 1978):

$$\frac{240}{\pi Re}(1 + 0.138 Re^{0.792}) w_b^2 = \frac{2}{15} l \left(1 - \frac{\rho_p}{\rho_w}\right) g, \tag{5}$$

where $Re$ is the particle Reynolds number ($Re = l w_b / \nu$, with $\nu = 1 \cdot 10^{-6}$), $l$ is the particle size, $\rho_w$ is the density of sea water (set to $1.029\,\mathrm{kg\,m^{-3}}$), and $g$ is the gravitational constant ($9.81\,m\,s^{-2}$).

In our model, the rise velocities are estimated assuming an ellipsoidal shape, with a density $\rho_p$ of $950\,\mathrm{kg\,m^{-3}}$. This combination gives a good match with reported densities (Morét-Ferguson et al., 2010) of plastic particles, and observed rise velocities (Poulain et al., 2019), see figure S4. In Poulain et al. (2019) a particle equivalent length was used, for ellipsoids defined as $L_{eq} = \sqrt{L_1 L_2 / 4}$, where $L_1$ is the length and $L_2$ is the width. We assume that these are approximately equal ($L_1 \approx L_2$), to simplify the calculations in terms of a particle size $l$.

Taking a balance between the upward particle flux caused by buoyancy, and a Reynolds-averaged turbulent flux, results in an exponential profile for the amount of particles as a function of depth ($n(z)$):

$$n(z) \sim \exp(z w_b A_0^{-1}), \tag{6}$$

for $z \leq 0$, where $A_0$ is an eddy-viscosity parameter estimated using $A_0 = 1.5 u_{*w} \kappa H_s$ (Thorpe et al., 2003), with $u_{*w}$ being the water friction velocity, $\kappa = 0.4$ the von Karman constant, and $H_s$ the significant wave height (Kukulka et al., 2012).

Particles at different depths will be affected differently by Stokes drift. The influence of Stokes drift with depth, $v_{Stokes}(z)$, is estimated using the approach presented in Breivik et al. (2016), where the wave spectrum is approximated

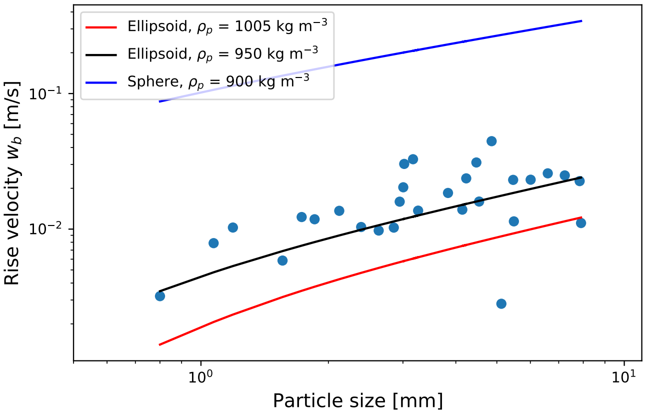


Figure S4: Estimated rise velocities using the model from Poulain et al. (2019). In Poulain et al. (2019) it was shown that most rise velocities of plastic particles fall in between those calculated for spheres ($900\,\mathrm{kg\,m^{-3}}$) and ellipsoids ($1005\,\mathrm{kg\,m^{-3}}$). Here, we use ellipsoids with $\rho_p = 950\,\mathrm{kg\,m^{-3}}$, which fit the measured rise velocities from Poulain et al. (2019) well, see the solid black line.

using the Phillips spectrum:

$$v_{Stokes}(z) = \frac{2\alpha g}{\omega_p}\left(\exp(2k_p z) - \sqrt{-2\pi k_p z}\,\mathrm{erfc}(\sqrt{-2k_p z})\right), \tag{7}$$

where $\alpha$ is Phillips' parameter ($8.3\cdot 10^{-3}$), $\omega_p$ is the wave peak frequency, and $k_p = \omega_p^2/g$ is the peak wavenumber.

ERA5 reanalysis data (Hersbach et al., 2020) is used to calculate typical weather conditions for the Mediterranean Sea. In order to evaluate the vertical mixing and the Stokes drift profiles, we need data for the peak wave period $\omega_p$, the significant wave height $H_s$, and the water friction velocity $u_{*w}$. The water friction velocity is estimated from the wind velocity at 10 meters $U_{10}$. First the air friction velocity $u_{*a}$ is estimated from the drag coefficient $C_D$ using (Thorpe et al., 2003; Geernaert, 1990):

$$u_{*a}^2 = C_D U_{10}^2,\ C_D = 10^{-3}\left(0.75 + 0.067\,U_{10}\,[m\,s^{-1}]\right), \tag{8}$$

afterwards continuous stress at the water surface is assumed, yielding

$$\rho_w u_{*w}^2 = \rho_a u_{*a}^2. \tag{9}$$

Statistics for $\omega_p$, $H_s$, and $U_{10}$ are plotted in figure S5. We calculate various quantiles from these data, in order to be able to evaluate the environmental box model for different weather conditions.

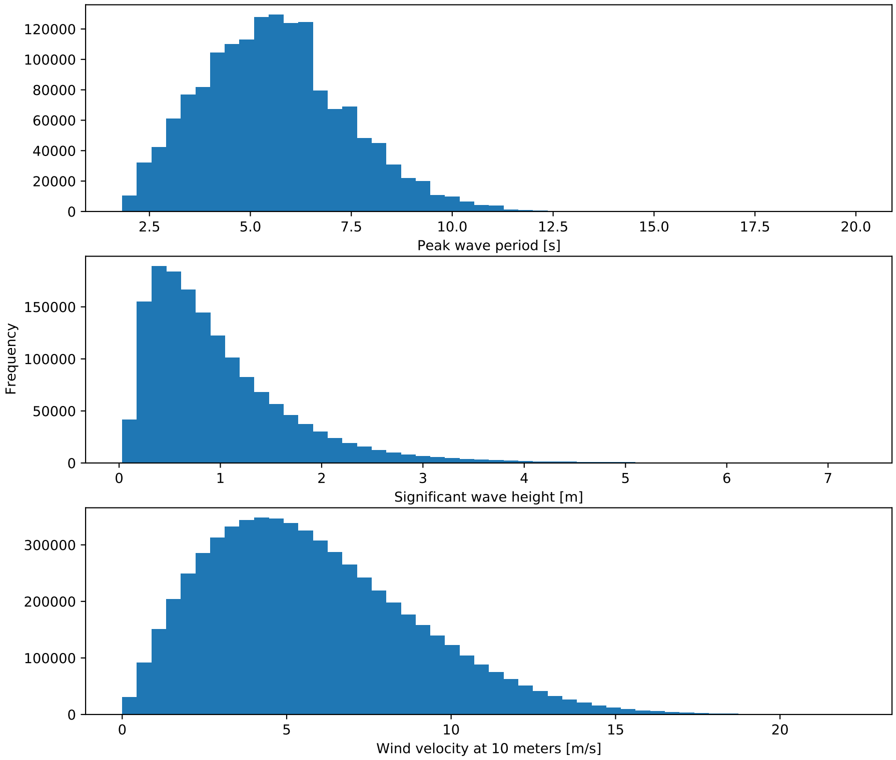


Figure S5: Wind and wave statistics for the Mediterranean, calculated from ERA5 reanalysis data (Hersbach et al., 2020)

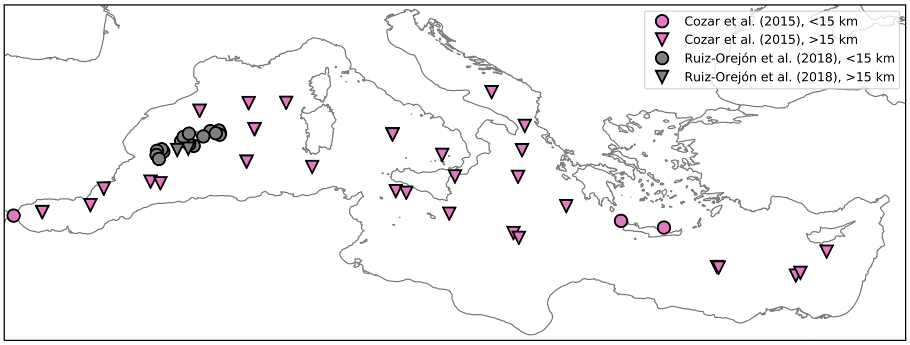


Figure S6: Dividing the ocean into a coastal region ($\leq$ 15 km from the coastline), and an open ocean region (> 15 km) divides the measurements from Cózar et al. (2015) and Ruiz-Orejón et al. (2018) quite well. The majority of samples from Cózar et al. (2015) are classified as open ocean this way (triangles), the majority of samples from Ruiz-Orejón et al. (2018) as coastal samples (circles). These measurements are used to compare the box model results with in the main text.

## S3.2 From mixing and Stokes drift to transition probabilities

In order to determine transition probabilities between the ocean and coastal water, we use the Lagrangian model run for the Mediterranean sea from Kaandorp et al. (2020). The domain of the Mediterranean Sea is split into offshore and coastal regions based on the distance to the closest coastline, with a threshold of 15 km. The 15 kilometer threshold was chosen as this divides the two sets of measurements by Ruiz-Orejón et al. (2018) (majority coastal samples) and Cózar et al. (2015) (majority offshore samples) well. This is shown in figure S6: coastal samples are plotted using dots, and offshore samples using triangles.

The Lagrangian particle simulation is run with the results found in Kaandorp et al. (2020) for five years starting from January the 1st 2010. From the total of approximately 770,000 particles, 66% are released based on the estimated mismanaged plastic waste at the coast (50 km radius)(Jambeck et al., 2015; SEDAC et al., 2015), 29% are released at river mouths based on Lebreton et al. (2017), and 6% are released at locations with high fishing activity (Kroodsma et al., 2018). Transition probabilities of particles moving between offshore and coastal cells of the mesh are calculated from this simulation.

The Stokes drift influence is varied in the simulation to estimate how this influences the transition probabilities between the ocean and coastal water. Six situations are simulated, ranging from no Stokes influence, to various fractions of Stokes drift, to full Stokes drift influence. These different situations can be translated to a certain depth, by evaluating the Stokes drift over depth using (7) and comparing this value to the surface Stokes drift (i.e. $\frac{v_{Stokes}(z)}{v_{Stokes}(0)}$) . Resulting

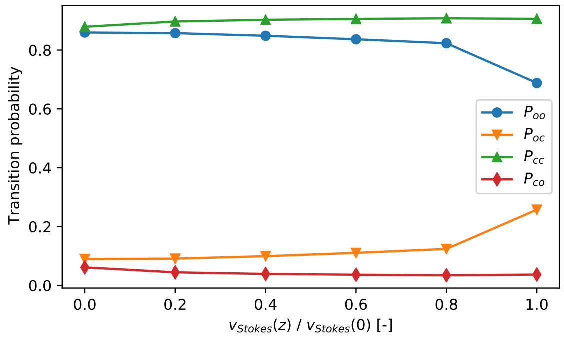


Figure S7: Transition probabilities between coastal and ocean cells for various values of $v_{Stokes}(z)$ / $v_{Stokes}(0)$ as calculated by the Lagrangian model run, for dt = 7 days

transition probabilities from the model runs are presented in figure S7. As can be seen, increasing the Stokes drift increases the probability that particles move from the ocean to coastal waters ($P_{O,C}$), decreases the probability that particles remain in the ocean ($P_{O,O}$), slightly increases $P_{C,C}$, and slightly decreases $P_{C,O}$ as expected. Even without Stokes drift, transport from the open ocean towards coastal waters can be observed. This accumulation of particles in the coastal zone means that the coastal transition probabilities are relatively insensitive to adding more Stokes drift.

Different particle sizes will be mixed to different depths using (5) and (6). The median depth of the particles is calculated, and the Stokes drift influence (i.e. the Stokes drift at this depth divided by the surface Stokes drift) is calculated using (7). This yields the results presented in figure S8. As wind speed and wave height increase (corresponding to increasing quantiles in figure S5), particles tend to be more mixed, and hence experience less Stokes drift.

Data in figure S7 are linearly interpolated for the Stokes drift influence at a given particle size as given in figure S8. This yields transition probabilities per particle size, results are presented in figure S9. These transition probabilities are used in the transition matrix of the environmental box model.

# S4 Estimated municipal plastic waste properties

Typical properties of municipal plastic waste were estimated using data from Jansen et al. (2015), in which waste mass fractions for different size classes were reported from sorting facilities in the Netherlands. Fine screen apertures are used (50-65 mm), midsize apertures (140 mm), and coarse apertures (220-250 mm) to sort the plastic waste. We take the midpoints here as the estimated aperture sizes (57.5 mm, 140 mm, and 235 mm). We assume the lower size limit to be 0 mm, and the upper size limit to be 500 mm, which is an arbitrary choice,

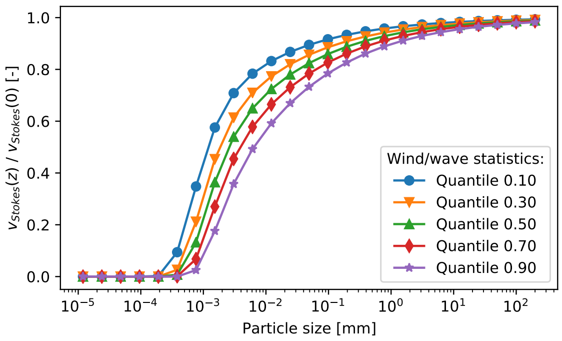


Figure S8: Stokes influence fraction (Stokes drift at a given depth divided by the surface Stokes drift, i.e. $v_{Stokes}(z)$ / $v_{Stokes}(0)$) for different particle sizes, under the influence of different wind/wave conditions presented in figure S5

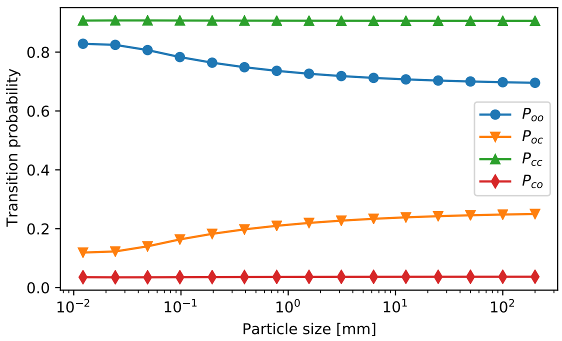


Figure S9: Transition probabilities for the environmental box model as a function of the particle size, calculated for the median wind/wave conditions

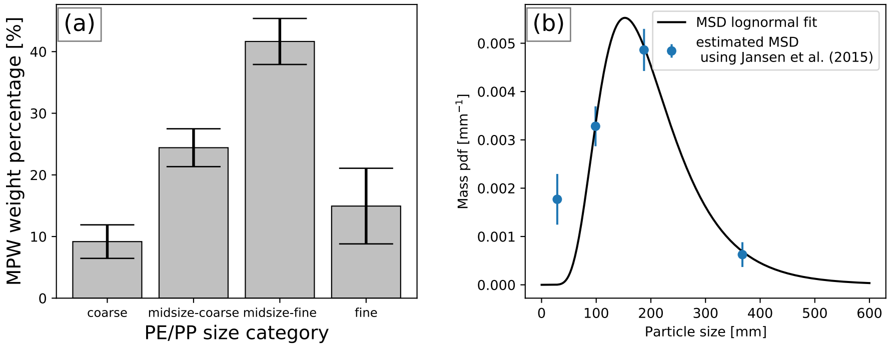


Figure S10: Quantification of municipal plastic waste dimensions, based on data from Jansen et al. (2015). Figure a: histogram of MPW masses reported for 4 different size categories. Figure b: estimated MSD using these data.

but does not have a large impact on the results. We use the reported mass data for polyethylene and polypropylene in Jansen et al. (2015), and use the environmental polymer fractions from Suaria et al. (2016) to estimate their contribution (76% and 24% respectively). Data are parsed using the WebPlotDigitizer tool Rohatgi (2020), and are shown in figure S10a.

We normalize the mass percentages by the bin widths, to obtain an estimate for the normalized MSD. The point estimates are given in figure S10b using the dots with errorbars. From this we argue that particles around 200 mm likely contribute to most of the new plastic mass entering the environment. Of course this is still a first order estimate, and more research is needed to quantify the mass, abundance, and dimensionality of 'new' plastics entering the environment. As an example we fit a lognormal distribution through the points in figure S10b, which fits the larger particle size classes well, but underestimates the smallest size class. It is important to further quantify the shape of this probability density function, since it will influence the particle size distributions measured in the environment.

# S5 Successive fragmentation model

In the main text we mention the fragmentation model by Cózar et al. (2014), which we will call the successive fragmentation model here. We summarise the basic details here, and the difference between the resulting NSD and normalized NSD.

Objects in the successive fragmentation model are successively broken down into a set of smaller (equally sized) fragments. Some iterations are shown in figure S11: a cube with a length of $L$ can be broken down into eight equally-sized smaller cubes with length $L/2$, which can again be broken down into 8

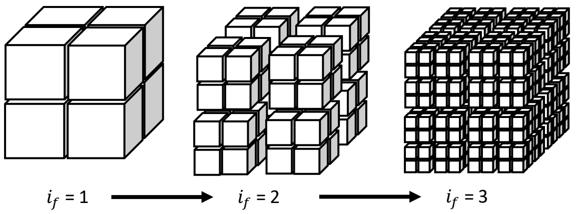


Figure S11: Illustration of the fragmentation model by Cózar et al. (2014)

smaller cubes with length $L/4$. A resulting histogram counting the amount of particles at fragmentation index $f$ is presented in figure S12.

The grey dashed line in figure S12 is obtained with a constant input rate of large objects with length $L = 1$ mm. The slope of this line on a log-log scale is -3. This slope is purely dependent of the spatial dimension considered for the fragmentation process. In case of the fragmentation of a 2-dimensional object (i.e. a square sheet with negligible thickness), this line would have a slope of -2 on a log-log scale. Results do not change when including a shape factor ($\alpha$, relating the volume ($V$) of the particles to their characteristic size ($l$) by $V = \alpha l^3$), and does not change when adjusting the amount of fragmentation events per iteration (which is 1 in this example).

This grey dashed line is not the resulting NSD however. It only connects the amount of fragments at a given discrete particle size. We can bin the amount of fragments per size class, e.g. using the bin boundaries as depicted by the vertical grey dotted lines. By dividing the amount of fragments in each bin by the width of the bin, we obtain the normalized abundance (red dashed line in figure S12), which is the particle size distribution normally reported in literature. Important to note is that the slope of this NSD is -4 instead of -3, due to the fact that the bin width decreases by a factor of two when going to the left on a log scale. This has been overlooked in e.g. Cózar et al. (2014), where NSD's with a slope of -3 were thought to be resulting from three-dimensional fragmentation, while in fact they correspond to two-dimensional fragmentation in the successive fragmentation model.

# References

Øyvind Breivik, Jean Raymond Bidlot, and Peter A.E.M. Janssen. A Stokes drift approximation based on the Phillips spectrum. *Ocean Modelling*, 100: 49–56, 2016. ISSN 14635003. doi: 10.1016/j.ocemod.2016.01.005.

R. Clift, J. R. Grace, and M. E. Weber. *Bubbles, Drops, and Particles.* Academic Press, 1978. ISBN 012176950X.

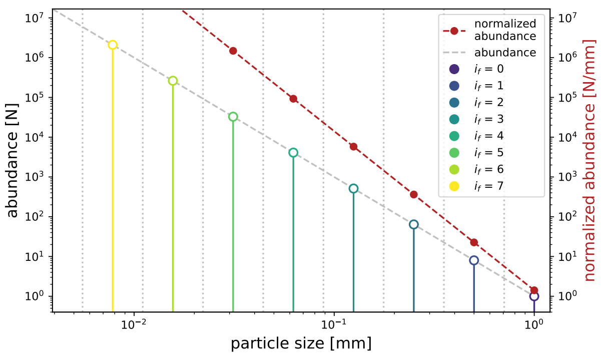


Figure S12: Illustration of the particle size distribution resulting from the successive breakage model


Andrés Cózar, Fidel Echevarría, J Ignacio González-Gordillo, Xabier Irigoien, Bárbara Ubeda, Santiago Hernández-León, Alvaro T Palma, Sandra Navarro, Juan García-de Lomas, Andrea Ruiz, María L Fernández-de Puelles, and Carlos M Duarte. Plastic debris in the open ocean. *Proceedings of the National Academy of Sciences of the United States of America*, 111 (28):10239–44, 2014. ISSN 1091-6490. doi: 10.1073/pnas.1314705111. URL `http://www.ncbi.nlm.nih.gov/pubmed/24982135%0Ahttp://www.pubmedcentral.nih.gov/articlerenc`

Andrés Cózar, Marina Sanz-Martín, Elisa Martí, J. Ignacio González-Gordillo, Bárbara Ubeda, José Á.gálvez, Xabier Irigoien, and Carlos M. Duarte. Plastic accumulation in the mediterranean sea. *PLoS ONE*, 10(4):1–12, 2015. ISSN 19326203. doi: 10.1371/journal.pone.0121762.

G.L. Geernaert. Bulk Parameterizations for the Wind Stress and Heat Fluxes. In G.L. Geernaert and W.J. Plant, editors, *Surface Waves and Fluxes*, pages 91–172. Kluwer Academic, 1990.

Hans Hersbach, Bill Bell, Paul Berrisford, Shoji Hirahara, András Horányi, Joaquín Muñoz-Sabater, Julien Nicolas, Carole Peubey, Raluca Radu, Dinand Schepers, Adrian Simmons, Cornel Soci, Saleh Abdalla, Xavier Abellan, Gianpaolo Balsamo, Peter Bechtold, Gionata Biavati, Jean Bidlot, Massimo Bonavita, Giovanna Chiara, Per Dahlgren, Dick Dee, Michail Diamantakis, Rossana Dragani, Johannes Flemming, Richard Forbes, Manuel Fuentes, Alan Geer, Leo Haimberger, Sean Healy, Robin J. Hogan, Elías Hólm, Marta Janisková, Sarah Keeley, Patrick Laloyaux, Philippe Lopez, Cristina Lupu, Gabor Radnoti, Patricia Rosnay, Iryna Rozum, Freja Vamborg, Sebastien Villaume, and Jean-Noël Thépaut. The ERA5 global reanalysis. *Quarterly Journal of the Royal Meteorological Society*, 146: 1999–2049, jul 2020. ISSN 0035-9009. doi: 10.1002/qj.3803. URL `https://onlinelibrary.wiley.com/doi/abs/10.1002/qj.3803`.

Jenna R Jambeck, Roland Geyer, Chris Wilcox, Theodore R Siegler, Miriam Perryman, Anthony Andrady, Ramani Narayan, and Kara Lavender Law. the Ocean. 347(6223), 2015.

M. Jansen, E.U. Thoden Van Velzen, and T. Pretz. *Handbook for sorting of plastic packaging waste concentrates*. Wageningen UR - Food & Biobased Research, 2015. ISBN 9789462575295.

Mikael L A Kaandorp, Henk A Dijkstra, and Erik van Sebille. Closing the Mediterranean Marine Floating Plastic Mass Budget : Inverse Modelling of Sources and Sinks. *Preprint*, 2020.

David A. Kroodsma, Juan Mayorga, Timothy Hochberg, Nathan A. Miller, Kristina Boerder, Francesco Ferretti, Alex Wilson, Bjorn Bergman, Timothy D. White, Barbara A. Block, Paul Woods, Brian Sullivan, Christopher Costello, and Boris Worm. Tracking the global footprint of fisheries. *Science*, 359(6378):904–908, 2018. ISSN 10959203. doi: 10.1126/science.aao5646.

T. Kukulka, G. Proskurowski, S. Morét-Ferguson, D. W. Meyer, and K. L. Law. The effect of wind mixing on the vertical distribution of buoyant plastic debris. *Geophysical Research Letters*, 39(7):1–6, 2012. ISSN 00948276. doi: 10.1029/2012GL051116.

Laurent C.M. Lebreton, Joost Van Der Zwet, Jan Willem Damsteeg, Boyan Slat, Anthony Andrady, and Julia Reisser. River plastic emissions to the world's oceans. *Nature Communications*, 8:1–10, 2017. ISSN 20411723. doi: 10.1038/ncomms15611. URL `http://dx.doi.org/10.1038/ncomms15611`.

Skye Morét-Ferguson, Kara Lavender Law, Giora Proskurowski, Ellen K. Murphy, Emily E. Peacock, and Christopher M. Reddy. The size, mass, and composition of plastic debris in the western North Atlantic Ocean. *Marine Pollution Bulletin*, 60(10):1873–1878, 2010. ISSN 0025326X. doi: 10.1016/j.marpolbul.2010.07.020.

Marie Poulain, Matthieu J Mercier, Laurent Brach, Marion Martignac, Corinne Routaboul, Emile Perez, Marie Christine Desjean, and Alexandra Halle. Small Microplastics As a Main Contributor to Plastic Mass Balance in the North Atlantic Subtropical Gyre. *Environmental Science & Technology*, 53:1157–1164, 2019. ISSN 0013-936X. doi: 10.1021/acs.est.8b05458.

Ankit Rohatgi. WebPlotDigitizer version 4.3, 2020. URL `https://automeris.io/WebPlotDigitizer`.

Luis F. Ruiz-Orejón, Rafael Sardá, and Juan Ramis-Pujol. Now, you see me: High concentrations of floating plastic debris in the coastal waters of the Balearic Islands (Spain). *Marine Pollution Bulletin*, 133(June):636–646, 2018. ISSN 18793363. doi: 10.1016/j.marpolbul.2018.06.010. URL `https://doi.org/10.1016/j.marpolbul.2018.06.010`.

SEDAC, CIESIN - Center for International Earth Science Information Network - Columbia University, FAO - United Nations Food and Agriculture Programme, and CIAT- Centro Internacional de Agricultura Tropical. Gridded Population of the World, Version 3 (GPWv3): Population Count Grid, 2015.

Giuseppe Suaria, Carlo G. Avio, Annabella Mineo, Gwendolyn L. Lattin, Marcello G. Magaldi, Genuario Belmonte, Charles J. Moore, Francesco Regoli, and Stefano Aliani. The Mediterranean Plastic Soup: Synthetic polymers in Mediterranean surface waters. *Scientific Reports*, 6:1–10, 2016. ISSN 20452322. doi: 10.1038/srep37551. URL http://dx.doi.org/10.1038/srep37551.

S. A. Thorpe, T. R. Osborn, D. M. Farmer, and S. Vagle. Bubble Clouds and Langmuir Circulation : Observations and Models. *Journal of Physical Oceanography*, 33(9):2013–2031, 2003.
